# Supplementary material for: pixelNeRF: Neural Radiance Fields from One or Few Images
Source: arXiv:2012.02190 source file (2021-05-30)
Supplement: Supplementary file 1 [file misc.tex]

\section{Miscellaneous}

\subsection{ShapeNet Category Name Abbreviations}

Abbreviations used are listed below.
Also note that we interchangeably use
airplane and plane.\\

    \begin{tabular}{@{}ll@{}}
\toprule
         Abbreviation &  Full Name  \\ \midrule
                cbnt. & cabinet \\
                disp. & display \\
                spkr. & speaker\\
\bottomrule
    \end{tabular}
    \vspace{1em}

\subsection{Things That Didn't Work}

In this section we discuss some things that were tried but didn't help in this project.
Future work may develop better solutions to the problems 
they were intended to address.

\paragraph{Camera frustum filtering}
A slight complication in our pixel-aligned approach is that for a point outside
an input view's frustum, no image feature information flows to the query point.
The previous approach \cite{PIFu} simply zeros out the image feature vector for such points,
while in our main paper we repeat the boundary features.
During our experiments, we tried a slightly more sophisticated solution: for each point, we only aggregate the image features from views for which it is inside the frustum.
For points not visible from any input view, we cannot expect a reasonable prediction and hence simply set $\sigma$ to zero.
 This process was implemented with a scatter operation.
However, we found that this only made results worse and created artifacts at the frustum boundaries.

\paragraph{Alpha regularization}
In our early experiments, we incorporated a
freespace regularization of \cite{NeuralVolumes} to try to clear up ``cloudy'' artifacts common to NeRF representations.
While this appeared to help when overfitting to single scenes,
it did not make a difference with the main models in ablations and was therefore removed.
