# Supplementary material for: pixelNeRF: Neural Radiance Fields from One or Few Images
Source: arXiv:2012.02190 source file (2021-05-30)
Supplement: Supplementary file 2 [file supplemental.tex]

\documentclass[final]{cvpr}
\usepackage[utf8]{inputenc}
\usepackage{graphicx}
\usepackage[dvipsnames]{xcolor}
\usepackage{color}
\usepackage{float}
\usepackage{booktabs}
\usepackage{amsmath}
\usepackage{amssymb}
\usepackage{multirow}
\usepackage{caption}
\usepackage{subcaption}
\usepackage{placeins}
\usepackage{paralist}
\usepackage{xr-hyper}
\usepackage[pagebackref=true,breaklinks=true,colorlinks,bookmarks=false]{hyperref}
\usepackage{times}

\include{commands}

 % *** Enter the CVPR Paper ID here

\linktoexternaldocument{main}

\title{Supplementary Material for\\ pixelNeRF:  
Neural Radiance Fields from One or Few Images}

\author{
Anonymous CVPR 2021 Submission\\ Paper ID 1291
\vspace{1em}
}

\begin{document}

\renewcommand{\thesection}{\Alph{section}}

\maketitle

\textit{
In this supplementary document, we discuss implementation details and
provide additional results.
}

\input{supplemental/results}

\section{Reproducibility}

\input{supplemental/impl_details}
\input{supplemental/exp_details}

\FloatBarrier

{\small
\bibliographystyle{ieee_fullname}
\bibliography{egbib}
}

\end{document}
