# Supplementary material for: pixelNeRF: Neural Radiance Fields from One or Few Images
Source: arXiv:2012.02190 source file (2021-05-30)
Supplement: Supplementary file 3 [file gencat_sm.tex]

\setlength{\tabcolsep}{6.0pt}
\begin{tabular}{@{}cccc@{}}
\toprule
     & $\uparrow$ PSNR & $\uparrow$ SSIM & $\downarrow$ LPIPS \\ \midrule
DVR  & 17.72          & 0.716          & 0.240           \\
SRN  & 18.71          & 0.684          & 0.280           \\
Ours & \textbf{22.71} & \textbf{0.825} & \textbf{0.182}  \\ \bottomrule
\end{tabular}
